# Supplementary material for: Adjusting for Autocorrelated Errors in Neural Networks for Time Series
Source: arXiv:2101.12578 source file (2021-10-08)
Supplement: Supplementary file 1 [file tanh_residual_appendix.tex]

\begin{figure}[h!]
\centering
\includegraphics[width=0.6\columnwidth]{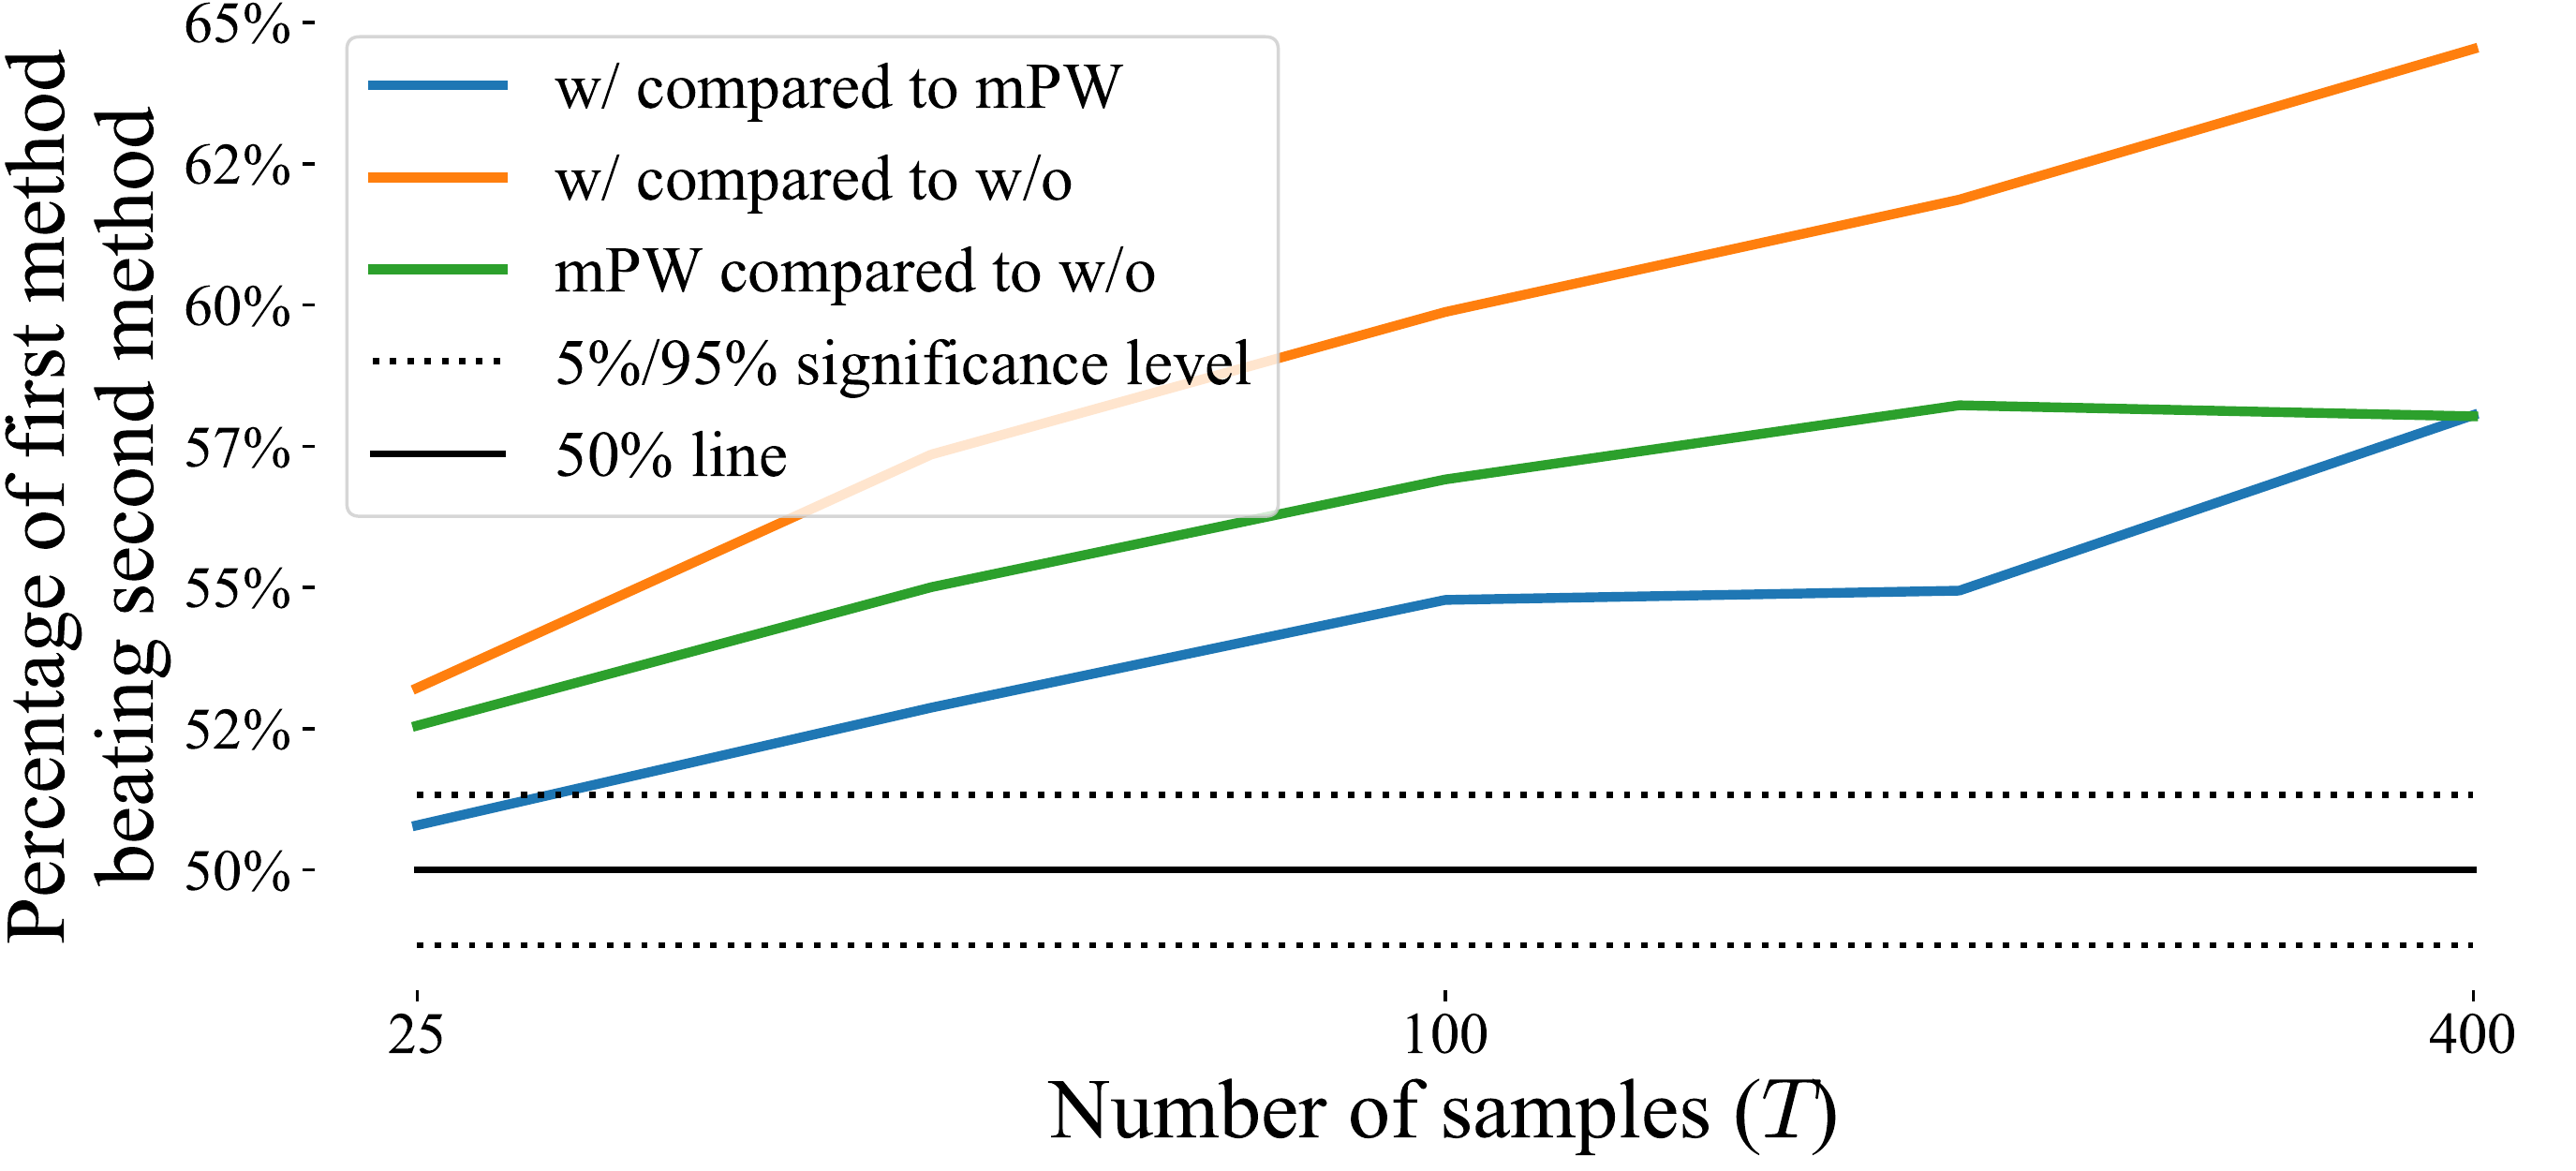}
\caption{Pairwise comparison of three methods of training NN on the synthesized data with different number of samples $T$. With more samples, the outperformance is more consistence, comparing to small-sample training where there are huge variances.}
\label{fig:tanh_residual_series_len}
\end{figure}

\begin{figure}[h!]
\centering
\includegraphics[width=0.6\columnwidth]{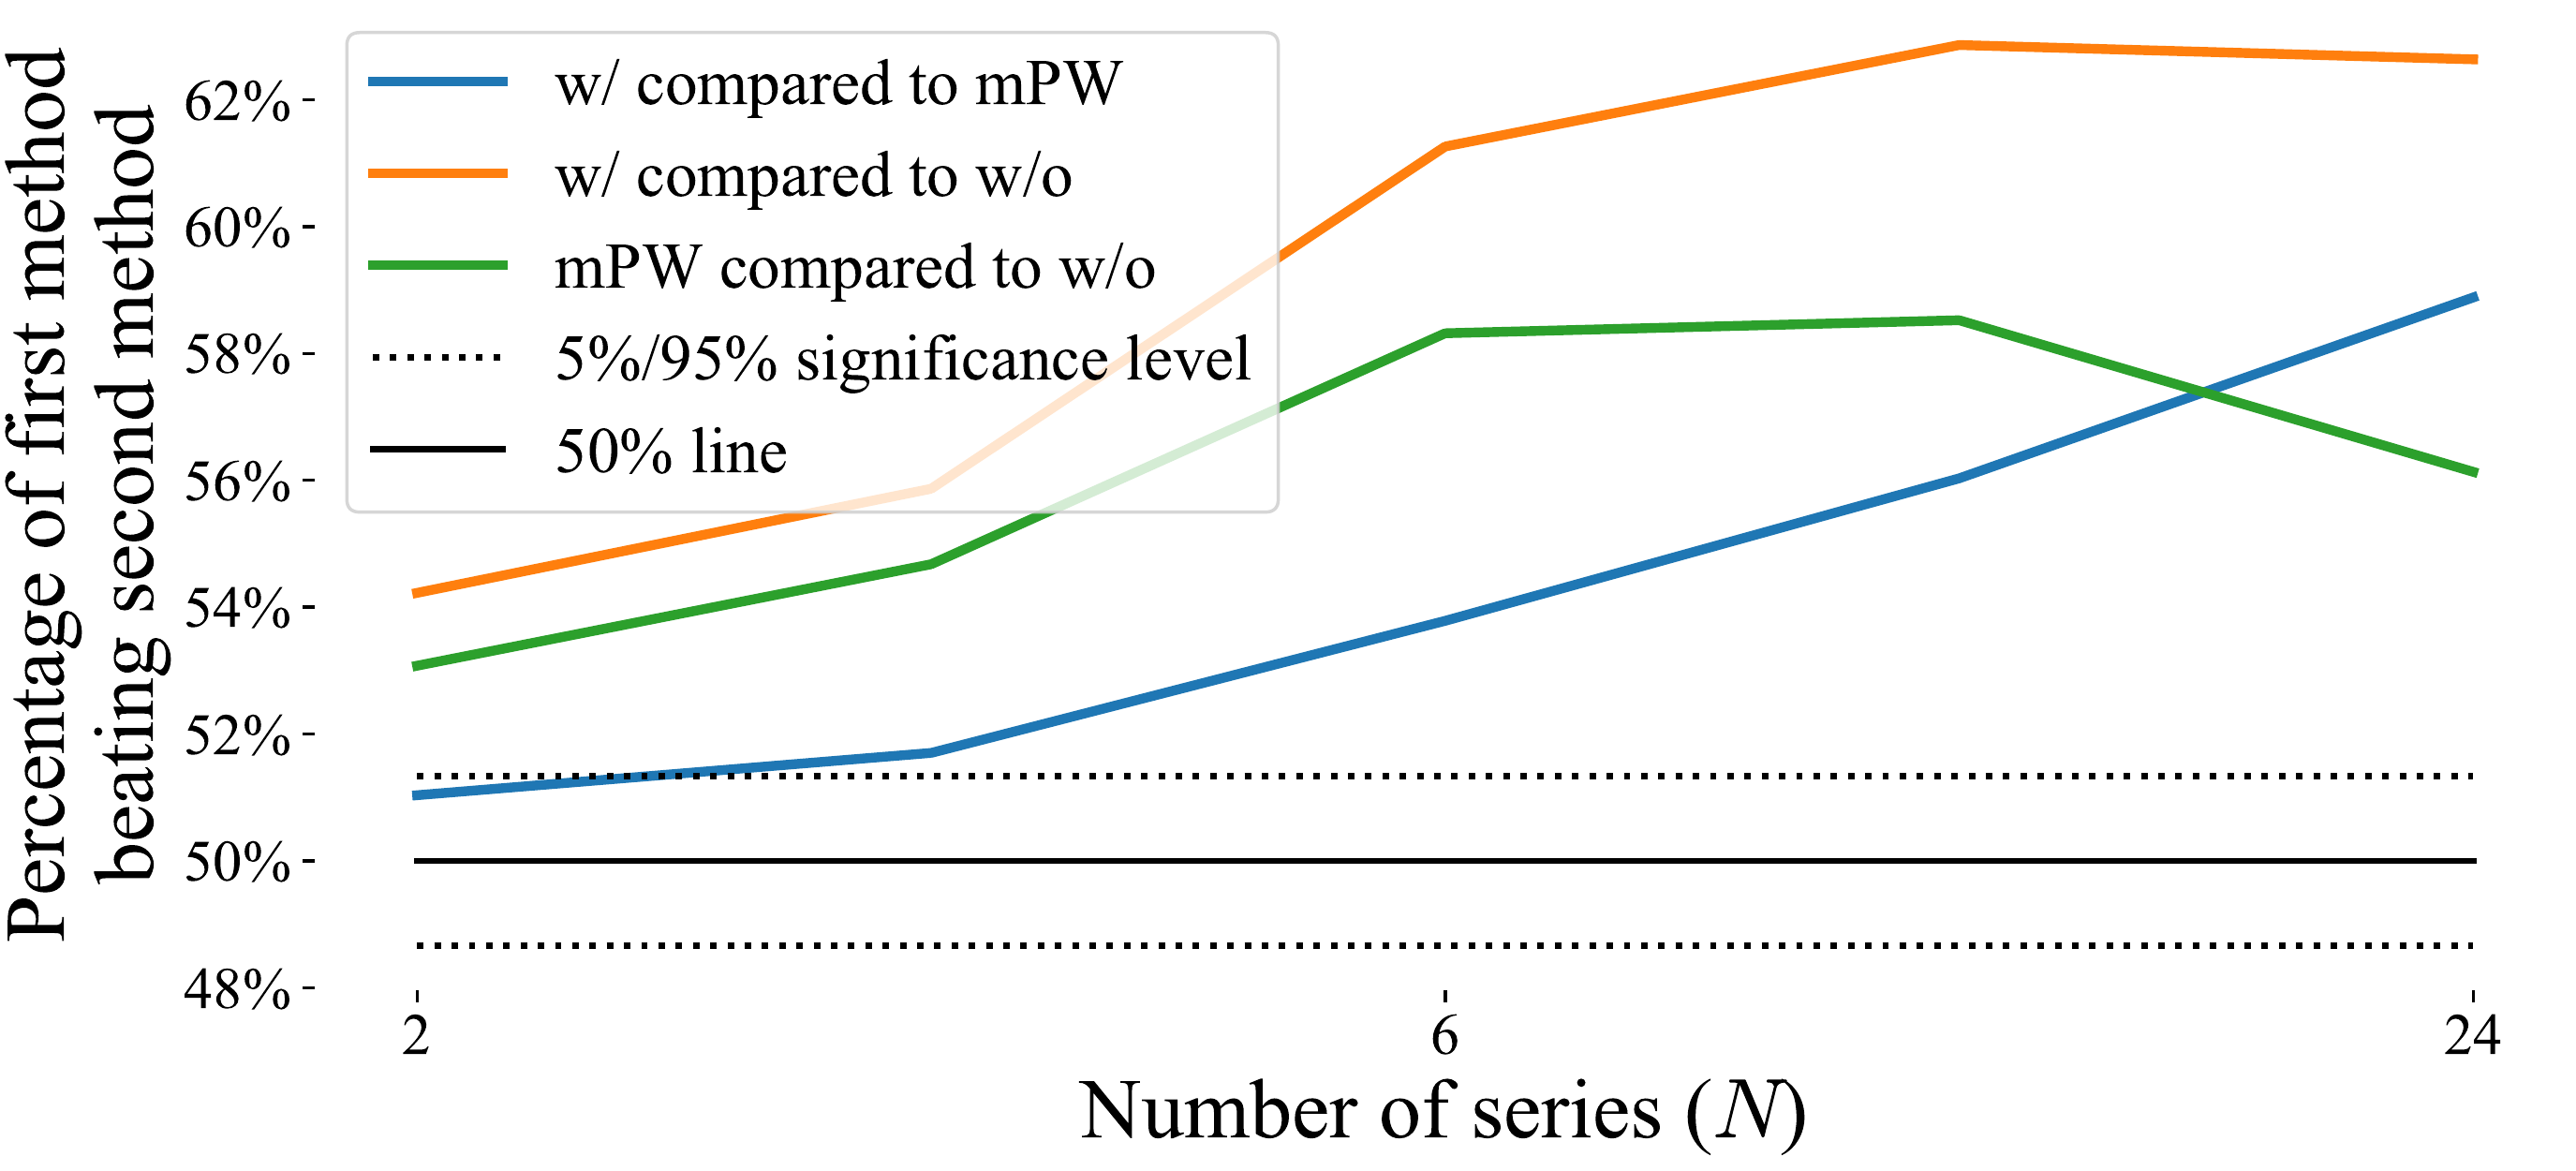}
\caption{Pairwise comparison of three methods of training NN on the synthesized data with different number of series $N$. With more series, more overfitting when autocorrelated errors are not adjusted.}
\label{fig:tanh_residual_n_series}
\end{figure}

\begin{figure}[h!]
\centering
\includegraphics[width=0.6\columnwidth]{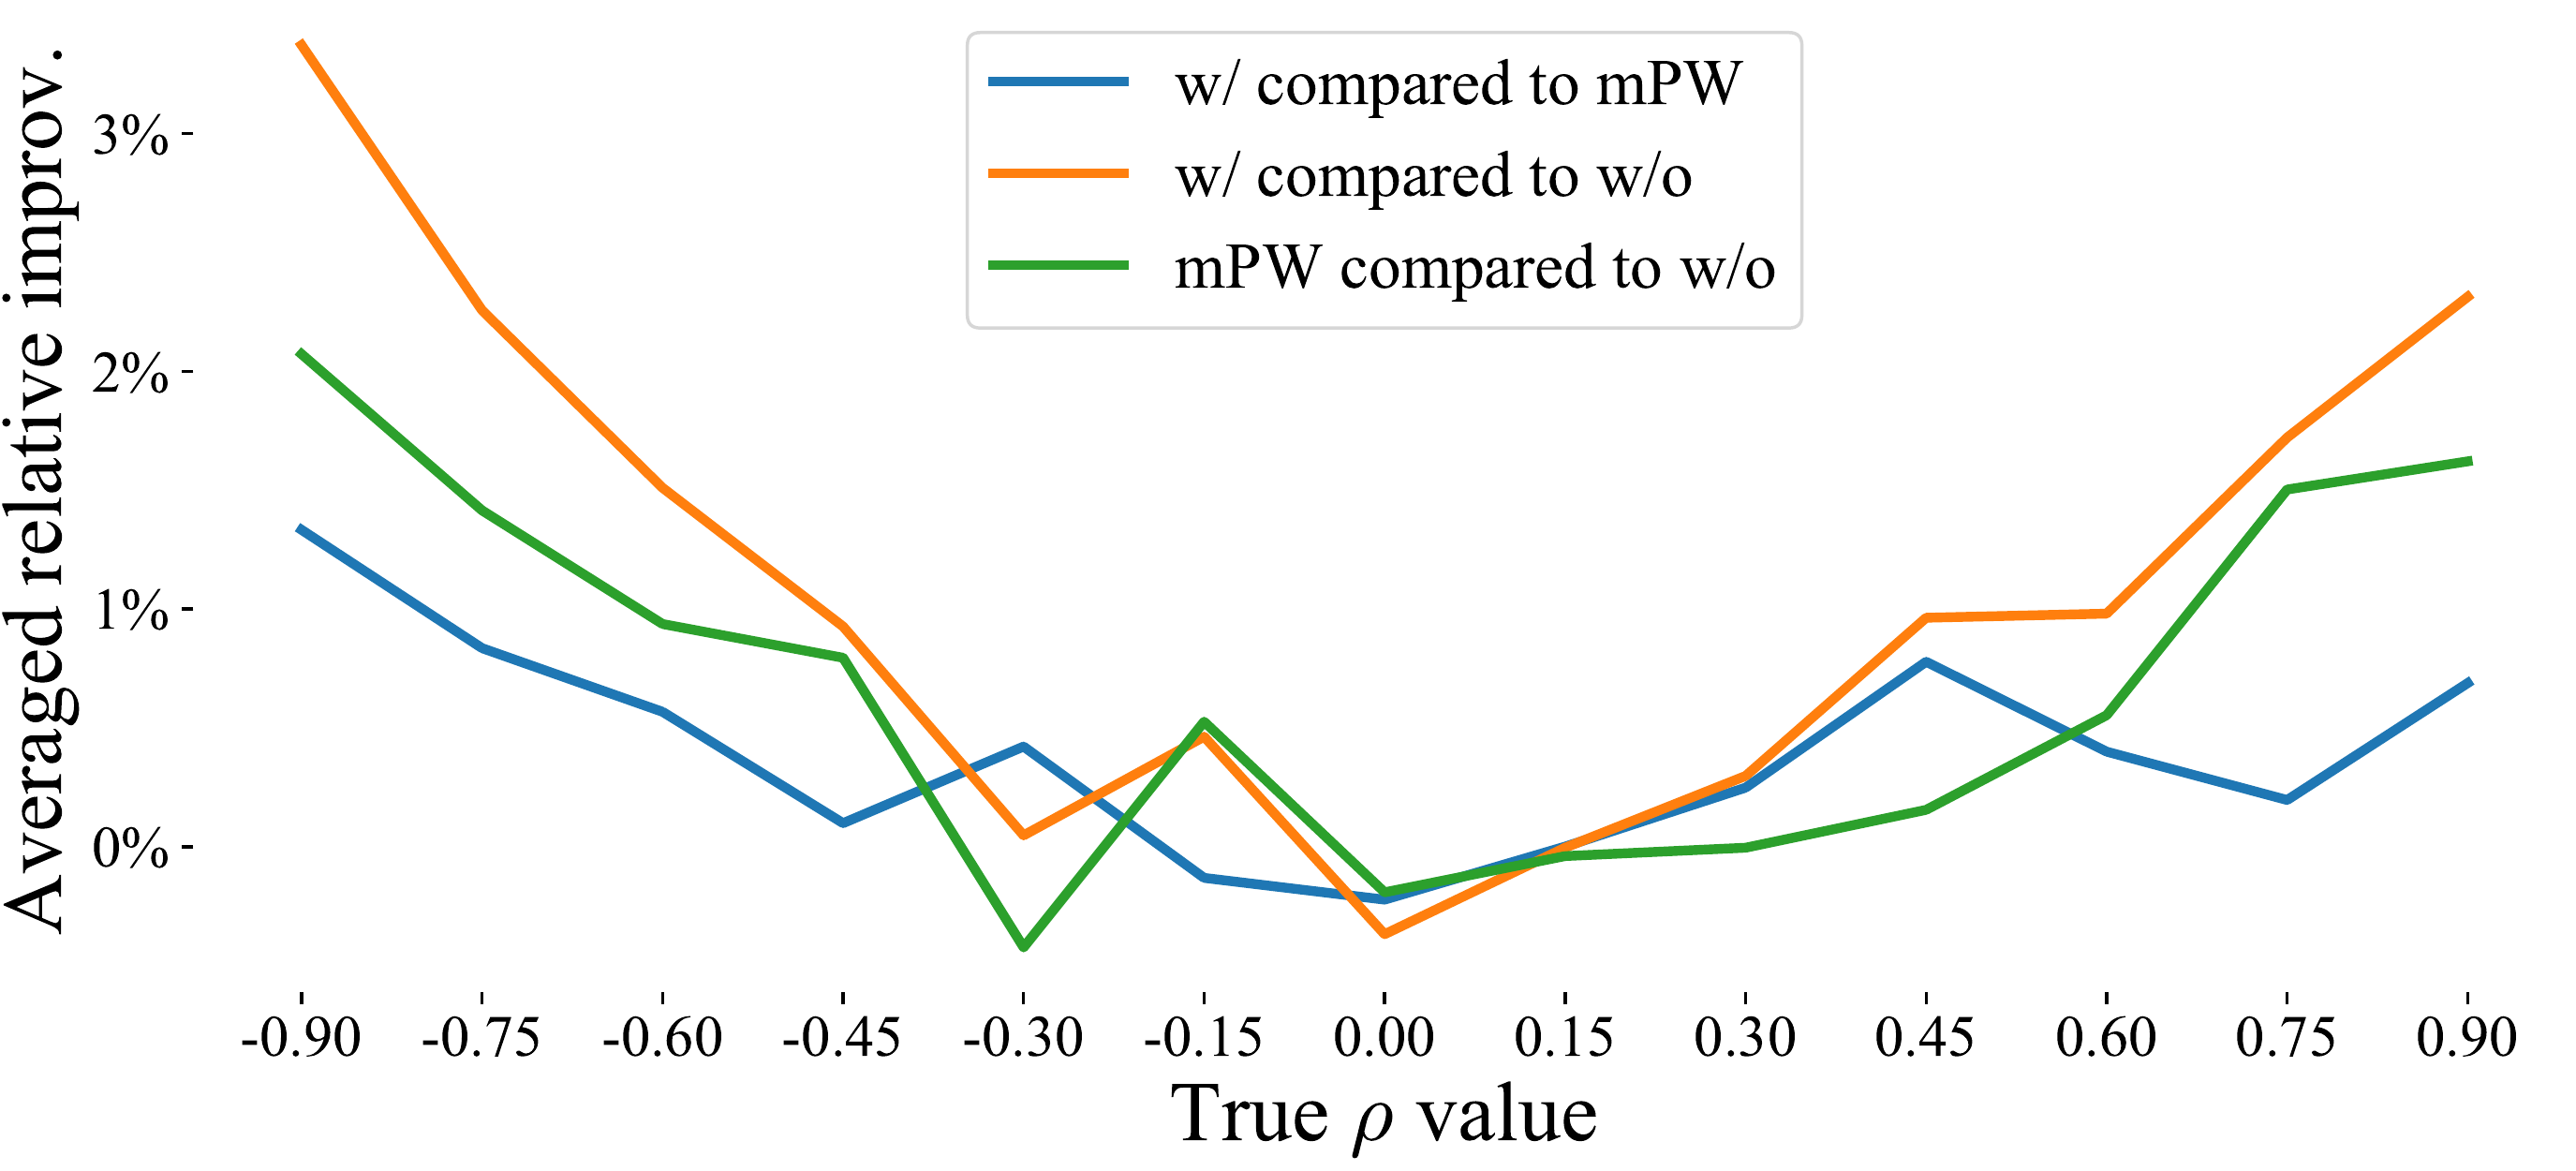}
\caption{Pairwise comparison of averaged relative improvement of three methods of training NN on the synthesized data with different true $\rho$ value. Results are similar to the one where $y$-axis is percentage of outperformance.}
\label{fig:tanh_residual_rho_rrsr}
\end{figure}

\begin{figure}[h!]
\centering
\includegraphics[width=0.6\columnwidth]{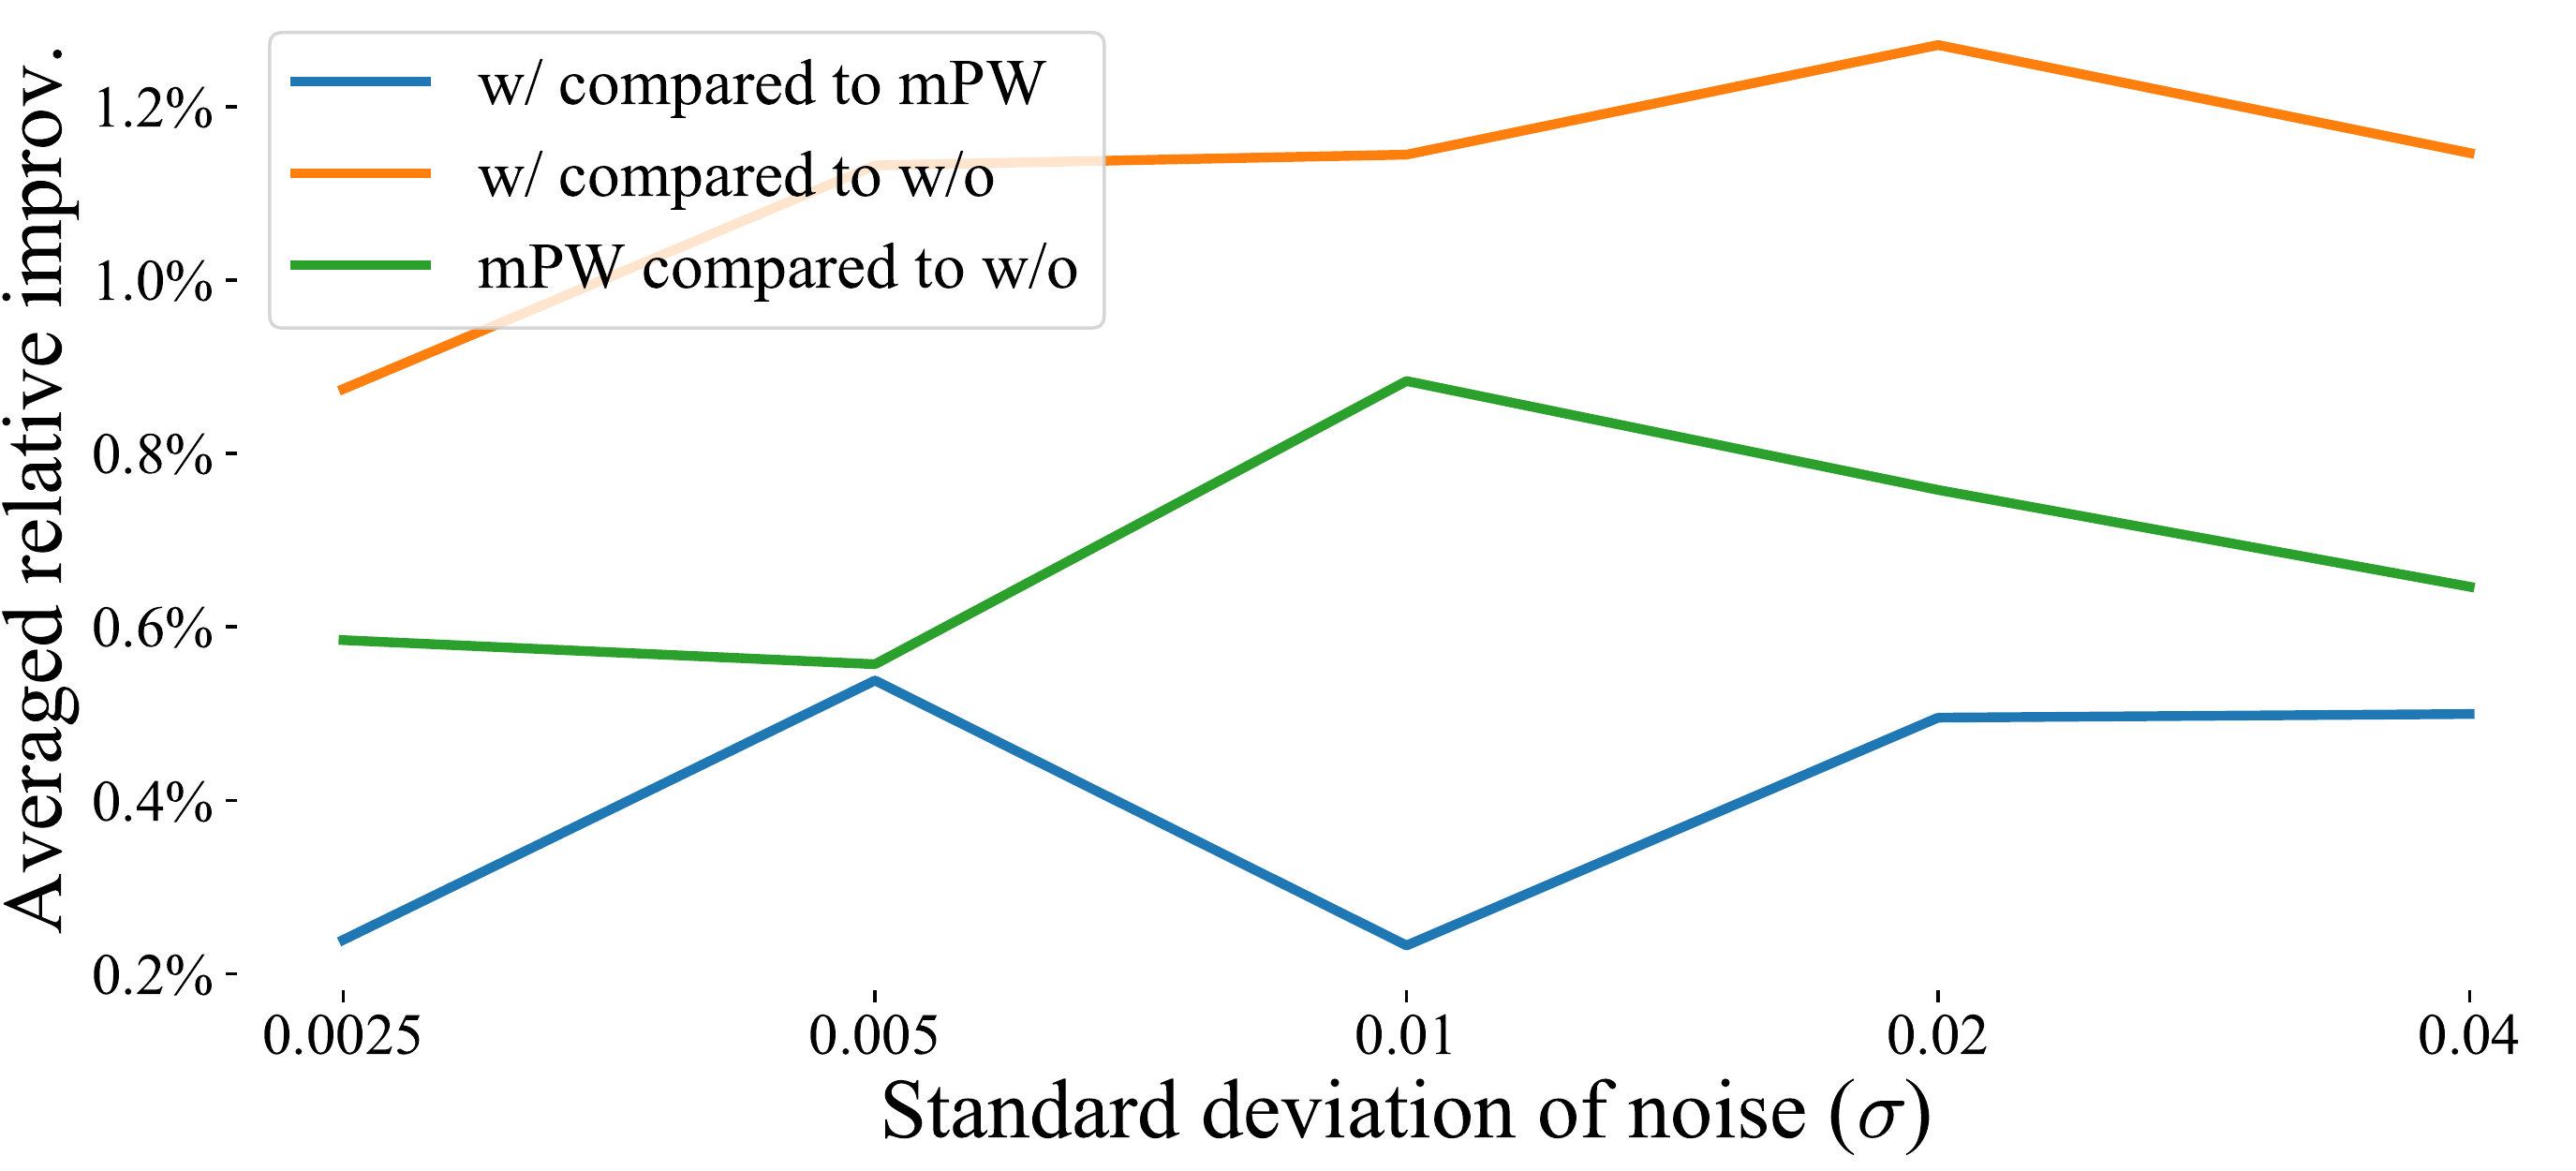}
\caption{Pairwise comparison of averaged relative improvement of three methods of training NN on the synthesized data with different standard deviation of noise ($\sigma$). Results are similar to the one where $y$-axis is percentage of outperformance.}
\label{fig:tanh_residual_noise_rrsr}
\end{figure}

\begin{figure}[h!]
\centering
\includegraphics[width=0.6\columnwidth]{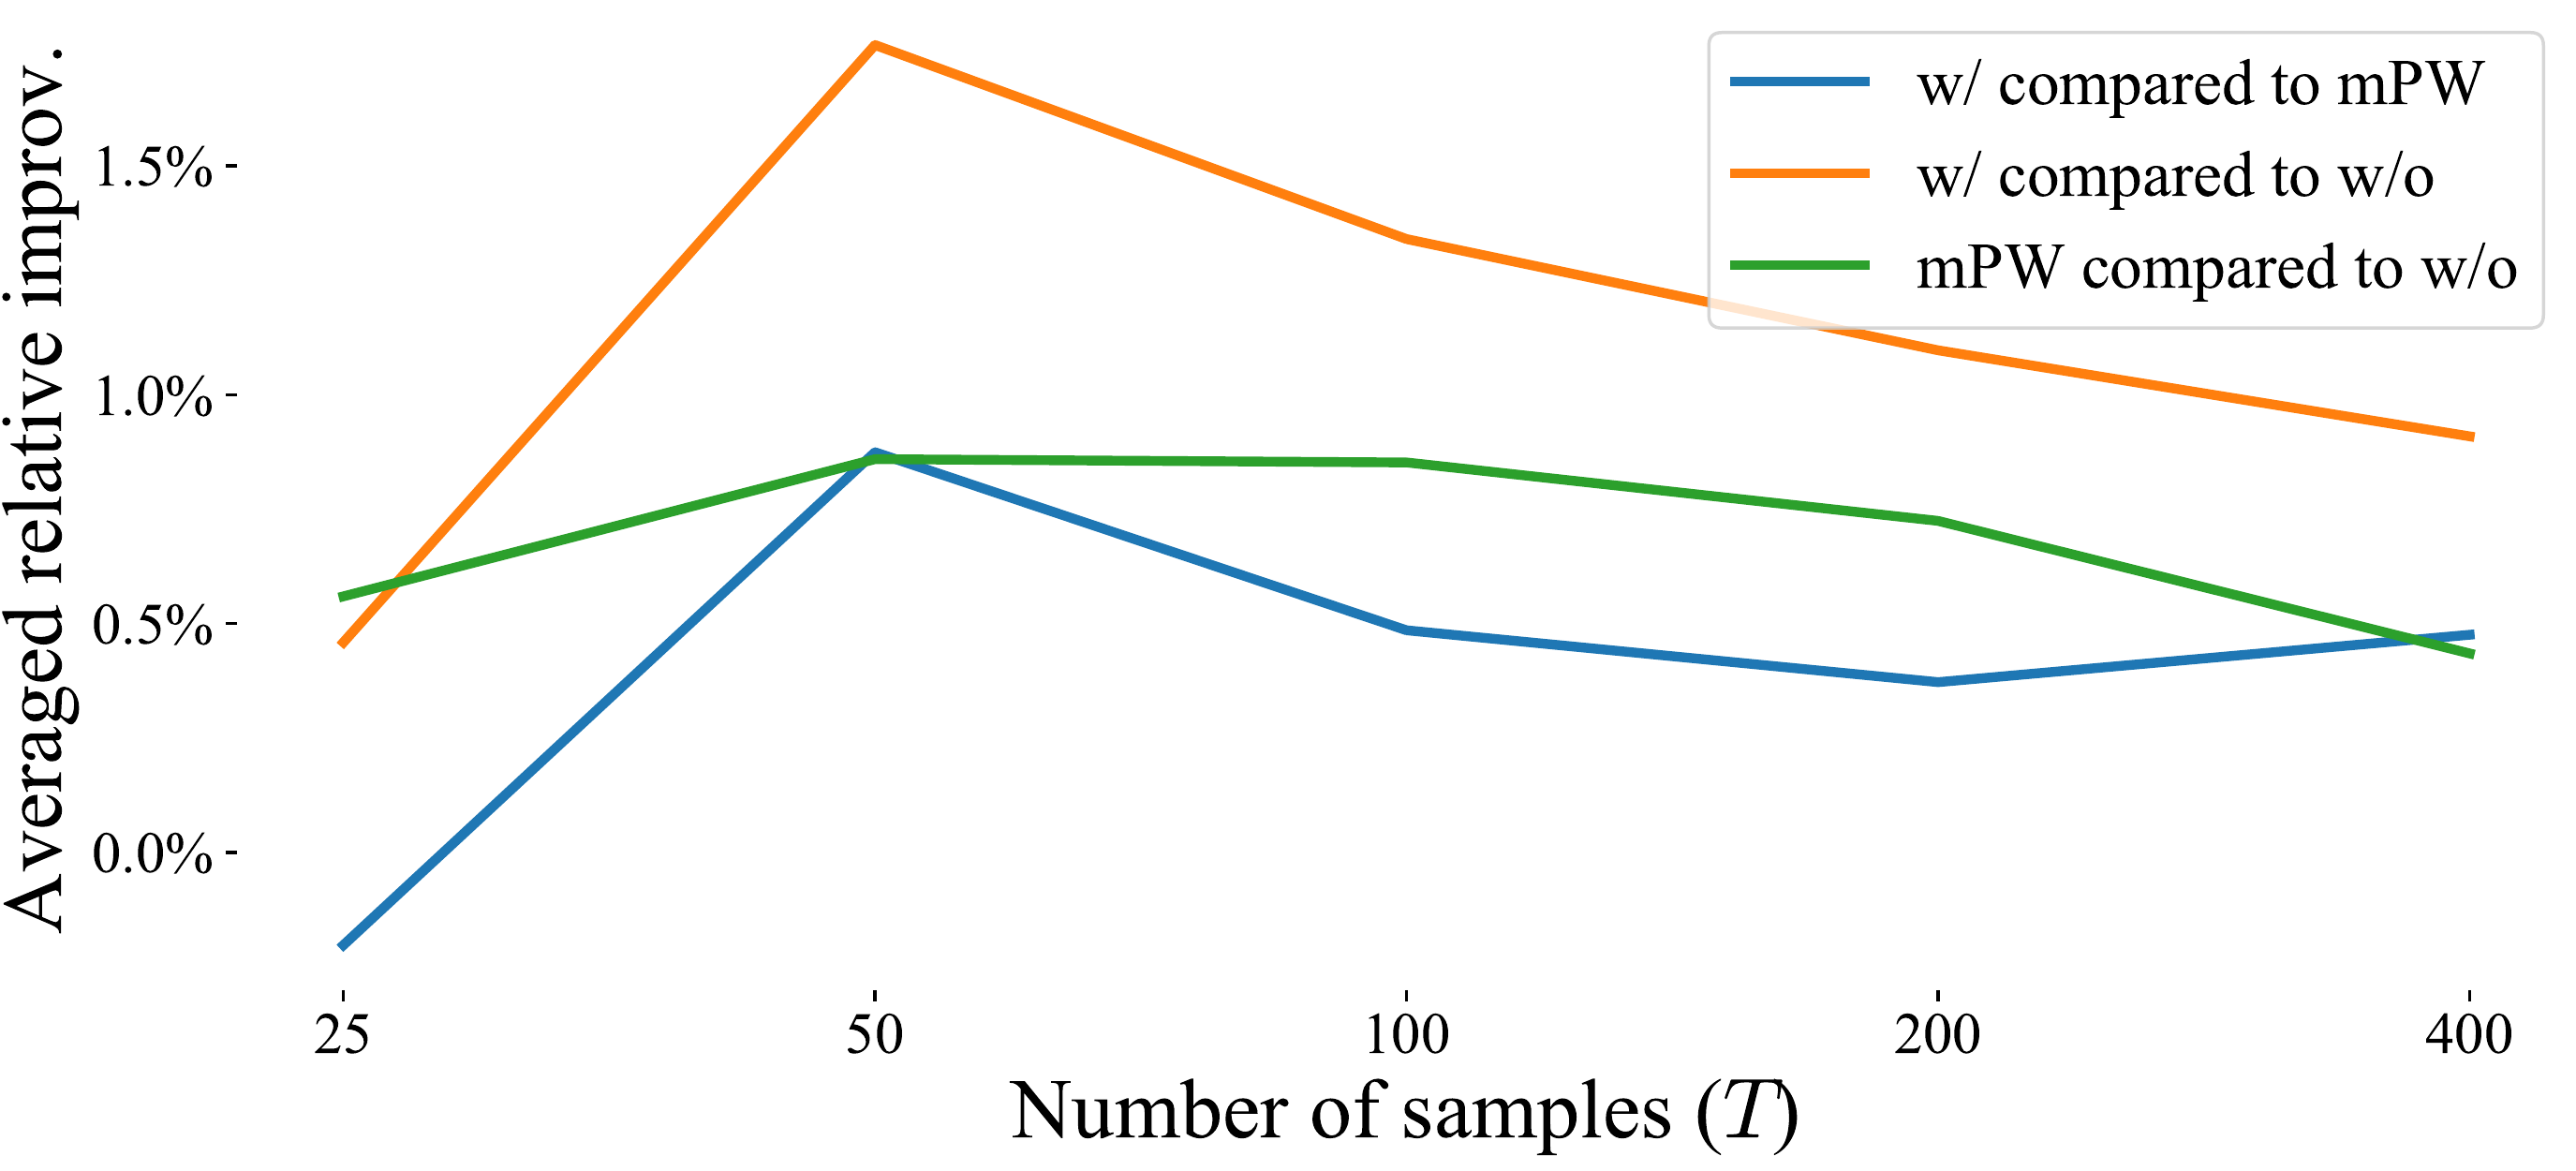}
\caption{Pairwise comparison of averaged relative improvement of three methods of training NN on the synthesized data with different number of samples ($T$). Results are similar to the one where $y$-axis is percentage of outperformance, except that when the number of samples increases, the improvement decreases because all methods have similar performances when number of samples approaches infinity.}
\label{fig:tanh_residual_series_len_rrsr}
\end{figure}

\begin{figure}[h!]
\centering
\includegraphics[width=0.6\columnwidth]{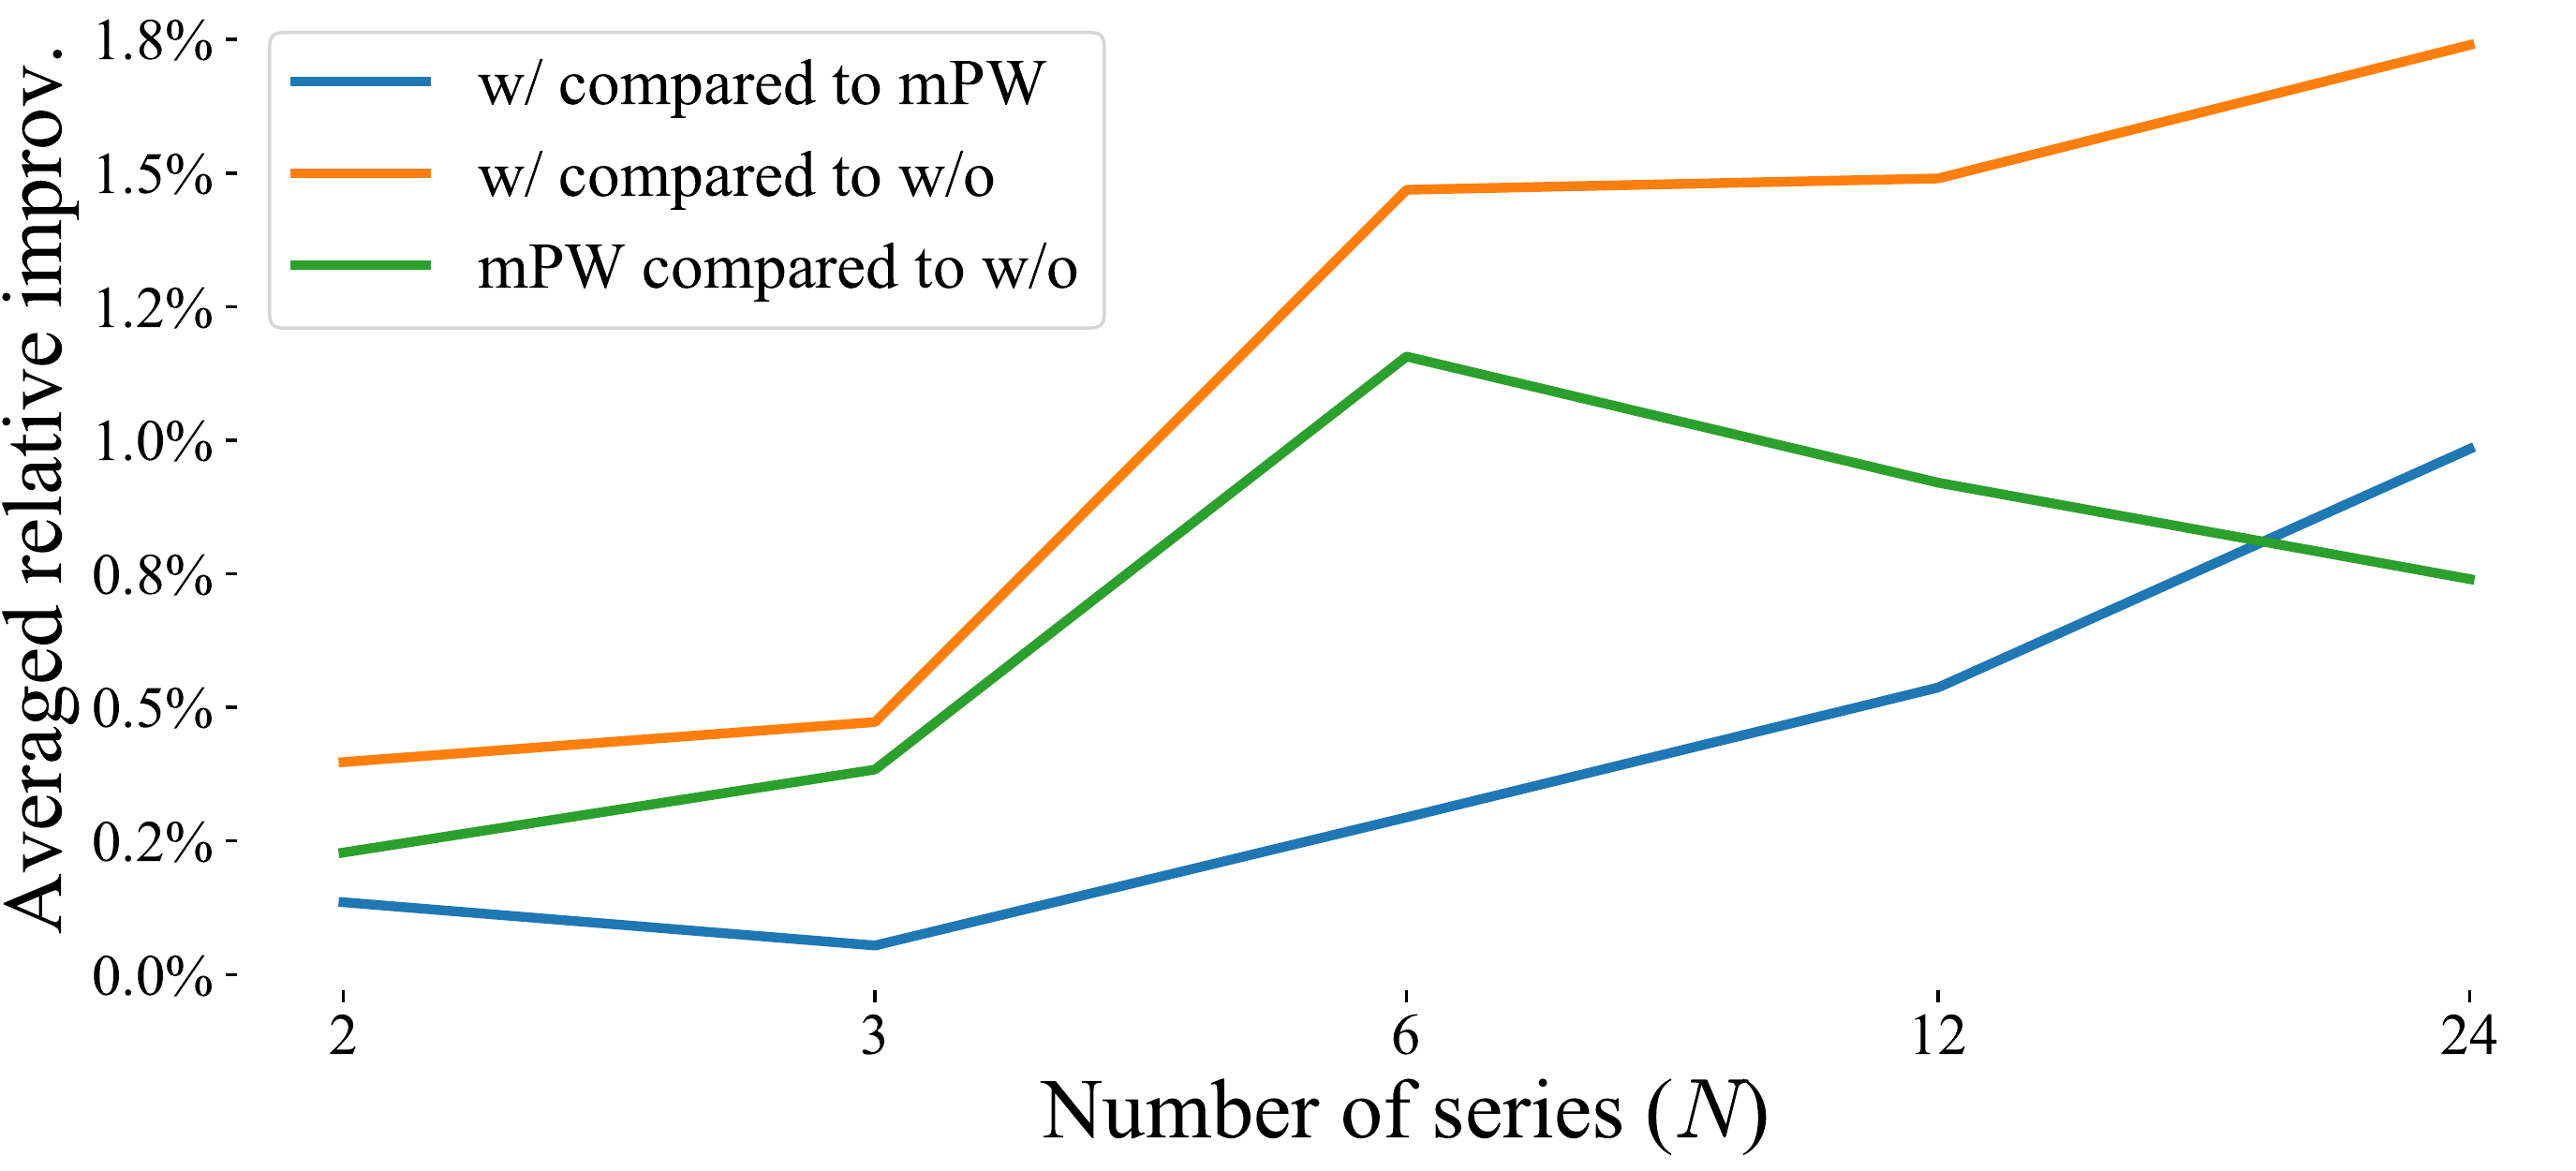}
\caption{Pairwise comparison of averaged relative improvement of three methods of training NN on the synthesized data with different number of series ($N$). Results are similar to the one where $y$-axis is percentage of outperformance.}
\label{fig:tanh_residual_n_series_rrsr}
\end{figure}
